# Supplementary material for: Regrading Policies for Flexible Information Flow Control in Session-Typed Concurrency
Source: arXiv:2407.20410 source file (2024-07-29)
Supplement: Supplementary file 2 [file abstract-syntax.tex]

\section{Abstract syntax}\label{apx:abstract-syntax}

\Cref{apx:fig:abstract-syntax} defines the abstract syntax of $\lang$.
Lines without a left-hand side are separated by $\alt$ from their preceding line.

\begin{figure*}
\begin{center}

\begin{tabular}{@{}llll@{}}
\\
\textbf{Sort} &
\phantom{$\defined$} &
\textbf{Abstract Form} &
\textbf{Remarks} \\
%%%
Metavariable & $\defined$
& $\Psi_0$ & concrete security lattice $\langle \mathcal{L}, \mc{E}_0, \sqcup, \sqcap \rangle$ \\
%%%
& & $\iota, \eta \in \mathcal{L}$ & set of concrete security levels \\
%%%
& & $\xi \in \mathcal{L}$ & concrete security level of observer \\
%%%
& & $E_0 \in \mathcal{E}_0$ & set of relations $E_0$ of form $\iota \sqsubseteq \iota'$ \\
%%%
& & $\Psi$ & security theory $\langle \mathcal{V}, \mathcal{E}, \sqcup, \sqcap \rangle$ \\
%%%
& & $\psi, \omega \in \mathcal{V}$ & set of security variables \\ 
%%%
& & $c, d, e, f \in \mathcal{S}$ & security terms of $\Psi$ \\
%%%
& & $p \in \mathcal{S} \times \mathcal{S}$ & pair of security terms of $\Psi$ \\
%%%
& & $E \in \mathcal{E}$ & set of relations $E$ of form $c \sqsubseteq d$ \\
%%%
& & $x_\alpha, x_\beta, x_\gamma, x_\delta$ & channel \\
%%%
& & $x, y, z, u, v, w$ & channel varianle\\
%%%
& & $j, k, \ell \in I, L$ & set of labels \\
%%%
& & $\Delta, \Lambda$ & linear typing contexts(channels) \\
%%%
& & $\Omega$ & linear typing contexts (variables)\\
% %%%
% & & $\Gamma$ & linear security typing contexts (channels)\\
% %%%
% & & $\Xi$ & linear security typing contexts(variables) \\
%%%
& & $K$ & linear typing context singleton(channel) \\
% %%%
% & & $K^s$ & linear security typing context singleton(channel) \\
%%%
% & & $\gamma_{\m{sec}}, \hat{\gamma_{\m{sec}}}, \delta_{\m{sec}}, \hat{\delta_{\m{sec}}}$ & order-preserving substitution of security elements \\
%%%
%& & $\mc{B}$ & closed process configuration \\
%%%
& & $\gamma, \hat{\gamma}, \delta, \hat{\delta}$ & channel var./ (order-pres.) label subst. \\
%%%
& & $ \mc{A}, \mc{B}, \mc{C}, \mc{D}, \mc{T}$ &  process configuration in $\lang$\\
% %%%
% % & & $ \mathbb{A}, \mathbb{B}, \mathbb{C}, \mathbb{D},  \mathbb{T}$ &  process configuration in $$\\
% & & $\gamma, \hat{\gamma}, \delta, \hat{\delta}$ & order-preserving substitution \\
% %%%
% & & $\mc{B}$ & closed process configuration \\
% %%%
% & & $\mc{C}, \mc{A}$ & open process configuration \\
%%%
% & & $\mc{P}(\mc{C})$ & a valid permutation of $\mc{C}$ \\
% %%%
% & & $\mnode, \mtree$ & program under consideration \\
% %%%
% & & $\substc, \substf$ & bottom and top closing contexts \\
%%%
Type $A, B, C, T$ & $\defined$
& $\intchoice{A}$ & internal choice, at least one label \\
%%%
& & $\extchoice{A}$ & external choice, at least one label \\
%%%
& & $\chanout{A}{B}$ & channel output \\
%%%
& & $\chanin{A}{B}$ & channel input \\
%%%
& & $\one$ & termination \\
%%%
& & $Y$ & type variable \\
%%%
Definition $X, Y$ & $\defined$
& $\procdefb{\D}{X}{P}{\psi_0}{\omega_0}{x}{A}{\psi}{\omega}$ & process definition \\
%%%
& & $Y = A$ & type definition \\
%%%
Process $P, Q$ & $\defined$
& $\labsnd{x}{k}{P}$ & label output \\
%%%
& & $\labrcv{x}{P}$ & label input \\
%%%
& & $\chnsnd{y}{x}{P}$ & channel output \\
%%%
& & $\chnrcv{y}{x}{P}$ & channel input \\
%%%
& & $\cls{x}$ & terminate process \\
%%%
& & $\wait{x}{Q}$ & wait for process to terminate \\
%%%
& & $\spwn{x}{c}{e}{X}{\D}{c_0}{e_0}{Q}$ & spawn \\
%%%
& & $\fwd{x}{y}$ & forward $x$ to $y$ \\
%%%
%%%
Messages $M,N$ & $\defined$
& $x.k$ & label output \\
%%%
& & $\mb{send}\, y\, x$ & channel output \\
%%%
& & $\cls{x}$ & terminate process 
\end{tabular}
\caption{Abstract syntax of $\lang$.}
\label{apx:fig:abstract-syntax}
\end{center}
\end{figure*}
