# Supplementary material for: Regrading Policies for Flexible Information Flow Control in Session-Typed Concurrency
Source: arXiv:2407.20410 source file (2024-07-29)
Supplement: Supplementary file 3 [file apx-logical-relation-i.tex]

\begin{small}
\[\begin{array}{lcl}
(1)\; ({\mc{D}_1};{\mc{D}_2}) &
\m{iff} &
( {\mc{D}_1} ; {\mc{D}_2} ) \in \m{Tree}(\cdot \Vdash y_\alpha)\, \m{and} \\
\qquad \in \mc{V}^c\llbracket \cdot \Vdash y_\alpha{:}1\rrbracket_{\cdot;y_\alpha}^{m+1} & & \mc{D}_1=\mathbf{msg}(\mathbf{close}\,y_\alpha ) \, \m{and}\, \mc{D}_2=\mathbf{msg}( \mathbf{close}\,y_\alpha)\\[4pt]
 
(2)\; ({\mc{D}_1} ; {\mc{D}_2}) &
\m{iff} &
({\mc{D}_1} ; {\mc{D}_2} ) \in \m{Tree}(\Delta \Vdash y_\alpha:\oplus\{\ell{:}A_\ell\}_{\ell \in I})\, \m{and}\,\,  \exists k_1,k_2 \in I.\\
 \qquad \in \mc{V}^c\llbracket (\Delta \Vdash y_\alpha{:}\oplus\{\ell{:}A_\ell\}_{\ell \in I})\rrbracket_{\cdot;y_\alpha}^{m+1}& & \mathcal{D}_1=\mathcal{D}'_1\mathbf{msg}(y_\alpha.k_1) \, \m{and}\, \mathcal{D}_2=\mathcal{D}'_2 \mathbf{msg}(y_\alpha.k_2)\, \m{and}\, k_1=k_2 \\
&& \m{and}\,({\mc{D}'_1};  {\mc{D}'_2}) \in  \mc{E}^c\llbracket \Delta \Vdash y_{\alpha+1}{:}A_{k_1}\rrbracket^{m}   \\[4pt]
   
(3)\; ({\mc{D}_1};{\mc{D}_2}) &
\m{iff} &
({\mc{D}_1}; {\mc{D}_2} ) \in \m{Tree}(\Delta \Vdash y_\alpha{:}\&\{\ell{:}A_\ell\}_{\ell \in I})\,\m{and}\,\,  \forall k_1, k_2 \in I.\,  \\
\qquad \in \mc{V}^c\llbracket \Delta \Vdash y_\alpha{:}\&\{\ell{:}A_\ell\}_{\ell \in I}\rrbracket_{y_\alpha; \cdot}^{m+1} && \mathbf{if}\, k_1=k_2\, \mathbf{then} ( {\mc{D}_1 \mathbf{msg}( y_\alpha.k_1)}; {\mc{D}_2\mathbf{msg}( y_\alpha.k_2)} )\in\\ && \quad \mc{E}^c\llbracket \Delta \Vdash y_{\alpha+1}{:}A_{k_1}\rrbracket^{m}    \\[4pt]
   
(4)\; ( {\mc{D}_1}; {\mc{D}_2})   &
\m{iff} &
( {\mc{D}_1} ;{\mc{D}_2} ) \in \m{Tree}(\Delta', \Delta'' \Vdash y_\alpha{:}A\otimes B)\, \m{and}\,\exists x_\beta\,\, \m{s.t.}\\
\qquad \in \mc{V}^c\llbracket \Delta',\Delta'' \Vdash y_\alpha{:}A\otimes B\rrbracket_{\cdot; y_\alpha}^{m+1}& &
\, \mathcal{D}_1=\mathcal{D}'_1\mathcal{T}_1\mathbf{msg}( \mb{send}\,x_\beta\,y_\alpha)\, \m{for}\, \mc{T}_1 \in \m{Tree}(\Delta'' \Vdash x_\beta{:}A)\, \m{and}\\
&& \mathcal{D}_2=\mathcal{D}'_2\mc{T}_2 \mathbf{msg}( \mb{send}\,x_\beta\,y_\alpha)\,\m{for}\, \mc{T}_2 \in \m{Tree}(\Delta'' \Vdash x_\beta{:}A)\, \m{and}\\
&& ( {\mc{T}_1}; {\mc{T}_2})  \in  \mc{E}^c\llbracket \Delta'' \Vdash x_{\beta}{:}A\rrbracket^{m} \,\m{and}\\
&& ( {\mc{D}'_1}; {\mc{D}'_2})  \in  \mc{E}^c\llbracket \Delta' \Vdash y_{\alpha+1}{:}B\rrbracket^{m}  \\[4pt]
  
(5)\; ( {\mc{D}_1} ; {\mc{D}_2} )&
\m{iff} &
( {\mc{D}_1}; {\mc{D}_2} ) \in \m{Tree}(\Delta \Vdash y_\alpha{:}A\multimap B)\, \m{and}\, \forall x_\beta {\not\in} \mathit{dom}(\Delta,y_\alpha{:}A \multimap B).\\
\qquad \in \mc{V}^c\llbracket \Delta \Vdash y_\alpha{:}A\multimap B\rrbracket_{y_\alpha; \cdot}^{m+1} && ( {\mc{D}_1\mathbf{msg}( \mb{send}\,x_\beta\,y_\alpha)};  {\mc{D}_2\mathbf{msg}(\mb{send}\,x_\beta\,y_\alpha)} )  \in \\
&&  \quad \mc{E}^c\llbracket \Delta, x_\beta{:}A\Vdash y_{\alpha+1}{:}B\rrbracket^{m}  \\[4pt]
   
(6)\; ({\mc{D}_1};{\mc{D}_2}) &
\m{iff} &
({\mc{D}_1}; {\mc{D}_2}) \in \m{Tree}(\Delta, y_\alpha{:}1 \Vdash K)\, \m{and} \\
\qquad \in\mc{V}^c\llbracket \Delta, y_\alpha{:}1 \Vdash K\rrbracket_{y_\alpha; \cdot}^{m+1}&&( {\mathbf{msg}( \mathbf{close}\,y_\alpha)\mc{D}_1}; {\mathbf{msg}( \mathbf{close}\,y_\alpha )\mc{D}_2} )\in \mc{E}^c\llbracket \Delta \Vdash K\rrbracket^{m}  \\[4pt]

(7)\; ( {\mc{D}_1} ; {\mc{D}_2} ) &
\m{iff} &
({\mc{D}_1} ; {\mc{D}_2} ) \in \m{Tree}(\Delta, y_\alpha{:}\oplus\{\ell{:}A_\ell\}_{\ell \in I} \Vdash K)\, \m{and}\, \forall k_1,k_2 \in I. \\
\qquad \in \mc{V}^c\llbracket \Delta, y_\alpha:\oplus\{\ell{:}A_\ell\}_{\ell \in I} \Vdash K\rrbracket_{y_\alpha; \cdot}^{m+1}&&\mathbf{if} \, k_1=k_2 \mathbf{then}\,({\mathbf{msg}(y_\alpha.k_1)\mc{D}_1}; {\mathbf{msg}(y_\alpha.k_2)\mc{D}_2}) \in\\
&& \quad  \mc{E}^c\llbracket \Delta, y_{\alpha+1}{:}A_{k_1} \Vdash K \rrbracket^{m} \\[4pt]
   
(8)\; ( {\mc{D}_1} ;{\mc{D}_2} )  &
\m{iff} &
({\mc{D}_1}; {\mc{D}_2} ) \in \m{Tree}(\Delta, y_\alpha{:}\&\{\ell{:}A_\ell\}_{\ell \in I} \Vdash K)\, \m{and} \, \exists k_1,k_2 \in I.\\
\qquad \in \mc{V}^c\llbracket \Delta, y_\alpha{:}\&\{\ell{:}A_\ell\}_{\ell \in I} \Vdash K \rrbracket_{\cdot; y_\alpha}^{m+1}\,  &&\mathcal{D}_1=\mathbf{msg}( y_\alpha.k_1) \mathcal{D}'_1 \, \m{and}\ \mathcal{D}_2=\mathbf{msg}( y_\alpha.k_2)\mathcal{D}'_2\,\m{and}\, k_1=k_2 \\
&&\m{and}\,({\mc{D}'_1}; {\mc{D}'_2}) \in  \mc{E}^c\llbracket \Delta, y_{\alpha+1}{:}A_{k_1} \Vdash K \rrbracket^{m} \\[4pt]
   
(9)\; ( {\mc{D}_1} ; {\mc{D}_2} )  &
\m{iff} &
( {\mc{D}_1} ; {\mc{D}_2} ) \in \m{Tree}(\Delta, y_\alpha{:}A\otimes B \Vdash K)\,\m{and}\, \forall x_\beta {\not \in} \mathit{dom}(\Delta,y_\alpha{:} A \otimes B, K). \\
\qquad  \in \mc{V}^c\llbracket \Delta, y_\alpha{:}A\otimes B \Vdash K \rrbracket_{y_\alpha; \cdot}^{m+1}&&({\mathbf{msg}( \mb{send}x_\beta\,y_\alpha)\mc{D}_1}; {\mathbf{msg}( \mb{send}x_\beta\,y_\alpha)\mc{D}_2}) \in \\
&& \quad \mc{E}^c\llbracket \Delta,x_\beta{:}A, y_{\alpha+1}{:}B \Vdash K \rrbracket^{m}  \\[4pt]
  
(10)\; ( {\mc{D}_1} ; {\mc{D}_2} )  &
\m{iff} &
 ({\mc{D}_1} ; {\mc{D}_2}) \in \m{Tree}(\Delta', \Delta'', y_\alpha{:}A\multimap B \Vdash K) \,\m{and} \, \exists x_\beta\, \m{s.t.}\\
\qquad \in \mc{V}^c\llbracket \Delta', \Delta'', y_\alpha{:}A\multimap B \Vdash K \rrbracket_{\cdot;y_\alpha}^{m+1}&& \mathcal{D}_1=\mathcal{T}_1\mathbf{msg}( \mb{send}x_\beta\,y_\alpha)\,\mathcal{D}''_1 \,\m{for}\, \mc{T}_1 \in \m{Tree}(\Delta' \Vdash x_\beta{:}A)\\
&& \mathcal{D}_2=\mathcal{T}_2\mathbf{msg}( \mb{send}x_\beta\,y_\alpha)\,\mc{D}''_2  \,\m{for}\, \mc{T}_2 \in \m{Tree}(\Delta' \Vdash x_\beta{:}A)\,\m{and} \\
&& ({\mathcal{T}_1};{\mathcal{T}_2}) \in  \mc{E}^c\llbracket \Delta' \Vdash x_\beta{:}A \rrbracket^{m} \,\m{and}\\
&&  ({\mc{D}''_1}; {\mc{D}''_2} ) \in  \mc{E}^c\llbracket \Delta'', y_{\alpha+1}{:}B \Vdash K \rrbracket^{m}\\[4pt]

(11)\; ({\mc{D}_1}; {\mc{D}_2}) \in\mc{E}^c\llbracket \Delta \Vdash K \rrbracket^{m+1} &
\m{iff} &
({\mc{D}_1}; {\mc{D}_2})\in \m{Tree}(\Delta \Vdash K)\,\m{and} \, \forall\, \Upsilon_1, \Theta_1, \mc{D}'_1.\, \m{if}\; {\mc{D}_1}\;\mapsto^{{*}_{\Upsilon_1; \Theta_1}}\; {\mc{D}'_1}\,\\ &&  \m{then}\,\exists \Upsilon_2, \mc{D}'_2 \m{\,such \, that\,}\,{\mc{D}_2}\mapsto^{{*}_{ \Upsilon_2}}{\mc{D}'_2},  \; \m{and}\, \Upsilon_1 \subseteq \Upsilon_2\; \m{and} \\[2pt]
&& \forall\, y_\alpha \in \mb{Out}(\Delta \Vdash K).\, \mb{if}\, y_\alpha \in \Upsilon_1.\, \mb{then}\, ({\mc{D}'_1}; {\mc{D}'_2})\in \mc{V}^c\llbracket  \Delta \Vdash K \rrbracket_{\cdot;y_\alpha}^{m+1}\,\m{and}\,\\[2pt]
&& \forall\, y_\alpha \in \mb{In}(\Delta \Vdash K). \mb{if}\, y_\alpha \in \Theta_1.\, \mb{then}\, ({\mc{D}'_1}; {\mc{D}'_2})\in \mc{V}^c\llbracket  \Delta \Vdash K \rrbracket_{y_\alpha;\cdot}^{m+1}
\\[4pt]
  
(12)\; ({\mc{D}_1}; {\mc{D}_2}) \in\mc{E}^c\llbracket \Delta \Vdash K \rrbracket^{0} &
\m{iff}&
({\mc{D}_1}; {\mc{D}_2})\in \m{Tree}(\Delta \Vdash K)

\end{array}\]%
\end{small}
